# Supplementary material for: Polarons from first principles
Source: arXiv:2512.06176 source file (2026-09-23)
Supplement: Supplementary file 1 [file SI.pdf]

# Supplemental Material: Polarons from first principles

Zhenbang Dai,[1,2,*] Jon Lafuente-Bartolome,[3,*] and Feliciano Giustino[1,2]
[1] *Oden Institute for Computational Engineering and Sciences, The University of Texas at Austin, Austin, Texas 78712, USA*
[2] *Department of Physics, The University of Texas at Austin, Austin, Texas 78712, USA*
[3] *Department of Physics, University of the Basque Country UPV/EHU, 48940 Leioa, Basque Country, Spain*

## CONTENTS

Supplemental Note 1: Connection between the Fröhlich and Landau-Pekar models
Supplemental Note 2: Polarons at finite density
Supplemental Note 3: Polaron hopping transport
Supplemental Note 4: Entanglement in the two-site Holstein model
Supplemental Note 5: Polarons at finite temperature
Supplemental Note 6: Bipolarons
Supplemental Note 7: Polarons out of equilibrium

* These authors contributed equally to this work.

## SUPPLEMENTAL NOTE 1: CONNECTION BETWEEN THE FRÖHLICH AND LANDAU-PEKAR MODELS

In this section, we outline the connection between the Fröhlich model reviewed in Sec. II.B and the Landau-Pekar model reviewed in Sec. II.A. This connection is helpful to contextualize the relation between the *ab initio* canonical transformation method (Sec. IV.A.1) and the *ab initio* polaron equations (Sec. VI.C).

To obtain the Landau-Pekar model starting from the Fröhlich Hamiltonian, Eq. (11), one considers a trial wavefunction in the form of a product state:

$$|\Psi\rangle = |\psi\rangle_{\rm el}\,|\chi\rangle_{\rm ph} \ , \tag{S1}$$

and represents the phonon wavefunction as a product of coherent states:

$$|\chi\rangle_{\rm ph} = \exp\sum_{\mathbf{q}}(\alpha_{\mathbf{q}}\hat{a}^\dagger_{\mathbf{q}} - \alpha^*_{\mathbf{q}}\hat{a}_{\mathbf{q}})\,|0\rangle_{\rm ph} \ . \tag{S2}$$

In this expression, symbols have the same meaning as in Sec. II; $|0\rangle_{\rm ph}$ represents the phonon vacuum, and the parameters $\alpha_{\mathbf{q}}$ are to be determined. The electronic part of the wave function can be expanded in Bloch states:

$$|\psi\rangle_{\rm el} = \frac{1}{\sqrt{N_p}}\sum_{\mathbf{k}} A_{\mathbf{k}}\hat{c}^\dagger_{\mathbf{k}}\,|0\rangle_{\rm el} \ , \tag{S3}$$

where $|0\rangle_{\rm el}$ represents the electron vacuum. Evaluating the expectation value of the Fröhlich Hamiltonian in Eq. (11) over the polaron wave function in Eqs. (S1)-(S3) gives:

$$\begin{aligned} E[\{A_{\mathbf{k}}\},\{\alpha_{\mathbf{q}}\}] &= \frac{1}{N_p}\sum_{\mathbf{k}}\varepsilon_{\mathbf{k}}|A_{\mathbf{k}}|^2 + \hbar\omega\sum_{\mathbf{q}}(|\alpha_{\mathbf{q}}|^2 + 1/2) \\ &+ \frac{1}{N_p^{3/2}}\sum_{\mathbf{k},\mathbf{q}} g(\mathbf{q})A^*_{\mathbf{k}+\mathbf{q}}A_{\mathbf{k}}(\alpha_{\mathbf{q}} + \alpha^*_{-\mathbf{q}}) \end{aligned} \tag{S4}$$

Variational minimization of this energy with respect to the coefficients $\alpha_{\mathbf{q}}$ yields:

$$\alpha_{\mathbf{q}} = -\frac{1}{N_p^{3/2}}\frac{g^*(\mathbf{q})}{\hbar\omega}\sum_{\mathbf{k}} A^*_{\mathbf{k}}A_{\mathbf{k}+\mathbf{q}} \ . \tag{S5}$$

Using this result inside (S4), one finds:

$$\begin{aligned} E[\{A_{\mathbf{k}}\}] &= \frac{1}{N_p}\sum_{\mathbf{k}}\varepsilon_{\mathbf{k}}|A_{\mathbf{k}}|^2 \\ &- \frac{1}{N_p^3}\sum_{\mathbf{q}}\frac{|g(\mathbf{q})|^2}{\hbar\omega}\left|\sum_{\mathbf{k}} A^*_{\mathbf{k}+\mathbf{q}}A_{\mathbf{k}}\right|^2 + \frac{\hbar\omega}{2}N_p. \end{aligned} \tag{S6}$$

The last term on the right-hand side is the contribution of the zero-point energy; since the Landau-Pekar model considers a classical polarization field, we ignore this term in the following. This expression can be recast in real space using the relation between the Fourier amplitudes $A_{n\mathbf{k}}$ and the wavefunction $\psi(\mathbf{r})$:

$$\psi(\mathbf{r}) = \frac{\Omega}{(2\pi)^3}\int d\mathbf{k}\,A_{\mathbf{k}}\,e^{i\mathbf{k}\cdot\mathbf{r}}, \tag{S7}$$

and the dispersion relation $\varepsilon_{\mathbf{k}} = \hbar^2|\mathbf{k}|^2/2m^*$:

$$\begin{aligned} E[\psi] &= \frac{\hbar^2}{2m^*}\int d\mathbf{r}|\nabla\psi(\mathbf{r})|^2 \\ &- \frac{\Omega}{(2\pi)^3}\int d\mathbf{q}\frac{|g(\mathbf{q})|^2}{\hbar\omega}\int d\mathbf{r}\int d\mathbf{r}' e^{i\mathbf{q}\cdot(\mathbf{r}-\mathbf{r}')}|\psi(\mathbf{r}')|^2|\psi(\mathbf{r})|^2 \ , \end{aligned} \tag{S8}$$

Using Eqs. (8) and (12) for the matrix element, one obtains the Landau-Pekar energy in Eq. (3).

## SUPPLEMENTAL NOTE 2: POLARONS AT FINITE DENSITY

*Ab initio* investigations of polarons at finite density and their collective behavior remain scarce, and only a few early attempts have been made at describing the polaron-driven metal-insulator transition (MIT). In its broadest sense, the MIT refers to the abrupt increase in electrical conductivity of a material in response to external parameters such as temperature, pressure, or doping (Imada *et al.*, 1998). MITs are well known in the study of doped semiconductors, where carriers remain bound to impurity states at low temperature; and in Mott insulators, where strong electron-electron correlations drive localization.

In the case of polarons, the methods reviewed in the main text primarily address the case of isolated polarons, that is an excess charge added to an otherwise insulating compound. In practice, a finite polaron density is unavoidable in experiments, therefore one might ask at which point polarons cease to exist as localized quasiparticles. Recent calculations (Dai and Giustino, 2024; Sio *et al.*, 2019a) investigated this questions by solving the *ab initio* polaron equations of Sec. VI.A as a function of polaron density; this was achieved by varying the size of the BvK supercell hosting a single polaron. Figure S1 shows that, for the case of LiF, there indeed exists a critical density above which localized polarons do not form. This effect is rationalized in terms of the spatial overlap between polaron wavefunctions belonging to different supercells, and is the polaron analog of the Mott transition in doped semiconductors (Mott, 1968).

While Fig. S1 captures certain features of the MIT in LiF, and shows semi-quantitative agreement with the Mott criterion (Sio *et al.*, 2019a), it is important to stress that such DFT supercell calculations do not describe a genuine phase transition. In fact, these calculations neglect both polaron-polaron interactions and the statistical mechanics of a polaron ensemble. A proper treatment of these collective aspects requires many-body ap-

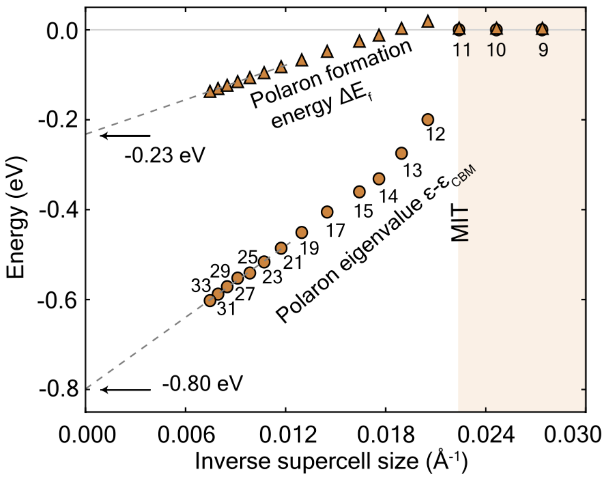


FIG. S1 Calculated MIT for electron polarons in LiF. Disks and triangles are polaron formation energy and eigenvalue, respectively. Polarons are stable (i.e., they have negative formation energy) for densities below the critical value $4{\cdot}10^{19}$ cm$^{-3}$, which marks the MIT. From Sio *et al.* (2019b).

proaches that explicitly incorporate electron-electron interactions. In this direction, recent advances such as dynamical mean-field theory applied to electron-phonon systems (Abramovitch *et al.*, 2025) and quantum Monte Carlo simulations of bipolaron condensates (Zhang *et al.*, 2023) offer promising new avenues.

## SUPPLEMENTAL NOTE 3: POLARON HOPPING TRANSPORT

The electron transfer rate given in Eq. (201) contains three parameters: the electronic transmission coefficient $\kappa$, the effective attempt frequency $\nu$, and the hopping energy barrier $E_{\rm a}$. The barrier is discussed in Sec. III.B; in this note, we elaborate on $\kappa$ and $\nu$.

Within the Landau-Zener theory (Landau, 1932b; Landau, 1932a; Zener, 1932; Newton, 1991), the electronic transmission coefficient is given by:

$$\kappa = 2P_{\rm LZ}/(1+P_{\rm LZ}), \tag{S9}$$

where $P_{\rm LZ}$ is the Landau-Zener transmission probability:

$$P_{\rm LZ} = 1 - e^{-2\pi\gamma} \ , \tag{S10}$$

and $\gamma$ is referred to as the adiabaticity parameter:

$$2\pi\gamma = \frac{\pi^{3/2} J^2}{2\pi\hbar\nu\sqrt{\lambda\, k_{\rm B}T}} \ . \tag{S11}$$

In this expression, $\lambda$ is the reorganization energy, and $J$ denotes the electronic coupling between neighboring sites. These quantities are illustrated schematically in the energy profile of a polaron hopping event in Fig. S2.

The reorganization energy $\lambda$ is defined as the vertical excitation energy between the initial and final diabatic surfaces, with the atomic configuration fixed at either state. Physically, it quantifies the energetic cost associated with structural reorganization of the lattice during charge transfer. It can be evaluated using constrained DFT (Wu and Ping, 2018), or, more simply, by approximating the diabatic energy surfaces as parabolas around the initial and final states (Lafuente-Bartolome *et al.*, 2024).

The electronic coupling (also called the transfer integral) $J$ measures the wavefunction overlap between neighboring sites, and thereby the probability of charge tunneling. This coupling is defined at the transition-state nuclear configuration, i.e. the atomic configuration where the diabatic potential energy surfaces of the initial and final charge-localized states intersect. This coupling has been computed using cluster models (Deskins and Dupuis, 2007), constrained DFT (Goldey *et al.*, 2017; Park *et al.*, 2018; Wu and Ping, 2018), or via the energy difference between the unoccupied and occupied KS states at the transition state (Adelstein *et al.*, 2014; Palermo *et al.*, 2024). In the simplest approximation, $J$ can also be inferred from the energy-difference between the crossing of the diabatic parabolas and the adiabatic energy barrier, as show in Fig. S2.

The effective attempt frequency $\nu$ can be computed within transition state theory (Eyring, 1935) using the vibrational partition functions in the initial configuration, $Z_0$, and in the transition state configuration, $Z_{\rm TS}$ (Adelstein *et al.*, 2014; Wimmer *et al.*, 2008; Wu and Ping, 2018):

$$\nu = \frac{k_{\rm B}T}{2\pi\hbar}\frac{Z_{\rm TS}}{Z_0} \ . \tag{S12}$$

In the harmonic approximation, the partition function is written as:

$$Z_0 = \Pi_i\, 2\sinh\big(\hbar\omega_i^0/2k_{\rm B}T\big) \ , \tag{S13}$$

where $\omega_i^0$ denotes a vibrational eigenfrequency of the supercell with the polaron in the initial configuration, and the translational modes are excluded from the product. The corresponding expression for $Z_{\rm TS}$ contains frequencies $\omega_i^{\rm TS}$ evaluated at the maximum of the potential energy barrier; in this case, the soft modes corresponding to maximum of the energy surface is also removed from the product.

In the high-temperature limit, $k_{\rm B}T \gg 2\pi\hbar\nu$, Eqs. (S12)-(S13) simplify to:

$$\nu = \frac{\Pi_i\, \omega_i^0}{\Pi_i\, \omega_i^{\rm TS}}. \tag{S14}$$

Conversely, in the low-temperature limit, $k_{\rm B}T \ll 2\pi\hbar\nu$, one finds:

$$\nu = \frac{k_{\rm B}T}{2\pi\hbar}\exp\left(\frac{\Delta E_{\rm ZP}}{k_{\rm B}T}\right) \ , \tag{S15}$$

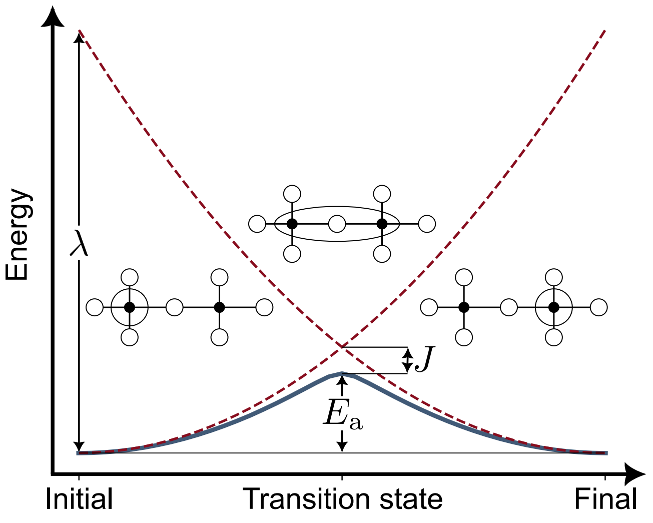


FIG. S2 Energy profile of polaron hopping process. The diabatic energy surfaces corresponding to the initial and final states are shown as dashed red lines, while the adiabatic energy surface is represented by the solid blue line. The inset provides a schematic representation of the atomic configurations associated with the initial, transition, and final states. Adapted from Deskins and Dupuis (2007) and Lafuente-Bartolome *et al.* (2024).

where $\Delta E_{\rm ZP} = \sum_i \hbar\omega_i^0/2 - \sum_i \hbar\omega_i^{\rm TS}/2$ is the difference in zero-point energies between the initial and the transition state.

Effective attempt frequencies have been computed from first principles using the above equations: Adelstein *et al.* (2014) and Wu and Ping (2018) employed phonon frequencies from supercell calculations at the Brillouin zone center; Carey *et al.* (2021); Falletta and Pasquarello (2023); and Palermo *et al.* (2024) employed an effective single-phonon approximation using the one-dimensional potential energy curve connecting the initial state to the transition state; Deskins and Dupuis (2007) and Lafuente-Bartolome *et al.* (2024) approximated the attempt frequency using the characteristic phonon mode driving polaron formation.

## SUPPLEMENTAL NOTE 4: ENTANGLEMENT IN THE TWO-SITE HOLSTEIN MODEL

We elaborate further on the two-site Holstein model of Sec. XI. We consider the Hamiltonian given by Eq. (207) and set $\epsilon = 0$, so that this Hamiltonian is invariant upon the exchange of the site indices 1 and 2.

It is advantageous to move to the center-of-mass frame of the oscillators, by introducing the sum and difference ladder operators via the canonical transformations $\hat{A} = (\hat{a}_1 + \hat{a}_2)/\sqrt{2}$ and $\hat{a} = (\hat{a}_2 - \hat{a}_1)/\sqrt{2}$. With these definitions, the Hamiltonian separates into $\hat{H} = \hat{H}_{\rm cm} + \hat{H}_{\rm rel}$, with:

$$\hat{H}_{\rm cm} = \hbar\omega \left(\hat{A} + g/\sqrt{2}\hbar\omega\right)^\dagger \left(\hat{A} + g/\sqrt{2}\hbar\omega\right) + \frac{\hbar\omega}{2} - \lambda t \,, \quad \text{(S16)}$$

$$\hat{H}_{\rm rel} = -t(c_1^\dagger c_2 + c_2^\dagger c_1) + \hbar\omega\left(\hat{a}^\dagger\hat{a} + \frac{1}{2}\right) + \frac{g}{\sqrt{2}}(\hat{a}^\dagger + \hat{a})\,(\hat{n}_2 - \hat{n}_1), \quad \text{(S17)}$$

where the definition of Holstein electron-phonon coupling strength from Eq. (31) has been used. The Hamiltonian $\hat{H}_{\rm cm}$ does not couple to the electron and is ignored in the following discussion. The ground state energy of this shifted oscillator is $E_{\rm cm,min} = \hbar\omega/2 - \lambda t$.

At strong coupling ($\lambda \to \infty$, while keeping the adiabaticity parameter $\hbar\omega/t$ fixed), the kinetic term in Eq. (S17) becomes negligible in comparison to the phonon and electron-phonon terms. In this limit, $\hat{H}_{\rm rel}$ reduces to a displaced harmonic oscillator precisely and its ground state energy is $E_{\rm rel,min} = \hbar\omega/2 - \lambda t$. Therefore, in the strong coupling limit, the ground state energy of the two-site Holstein model, $E_{\rm cm,min} + E_{\rm rel,min}$, tends to $\hbar\omega - 2\lambda t$, which is the same limit as the full Holstein model in Fig. 4 of the main text.

To analyze Eq. (S17) at any coupling strength, exact numerical diagonalization is straightforward; results for the site polarization are shown in Fig. 26. There are no closed-form solutions, but one can gain intuition into the nature of the eigenstates by expressing the ladder operators in the position representation and the electron site index in pseudospin representation. With this change of basis, the eigenvalue problem for $\hat{H}_{\rm rel}$ takes the form:

$$-\frac{\hbar^2}{2m}\frac{d^2}{dx^2}\chi_1 + \frac{1}{2}m\omega^2(x - x_0)^2\chi_1 - t\chi_2 = E\chi_1 \quad \text{(S18)}$$

$$-\frac{\hbar^2}{2m}\frac{d^2}{dx^2}\chi_2 + \frac{1}{2}m\omega^2(x + x_0)^2\chi_2 - t\chi_1 = E\chi_2 \quad \text{(S19)}$$

having used the standard relations for the quantum harmonic oscillator:

$$\hbar\omega\left(\hat{a}^\dagger\hat{a} + \frac{1}{2}\right) = -\frac{\hbar^2}{2m}\frac{d^2}{dx^2} + \frac{1}{2}m\omega^2 x^2 \,, \quad \hat{a} + \hat{a}^\dagger = \sqrt{\frac{2m\omega}{\hbar}}x \,. \quad \text{(S20)}$$

The mass $m$ is inconsequential and is kept for dimensional consistency. The functions $\chi_1(x)$ and $\chi_2(x)$ in Eqs. (S18)-(S19) describe the oscillator, and the electron degree of freedom is encoded in the pseudospin indices 1 and 2. The shift parameter $x_0$ is related to the Holstein electron-phonon coupling strength via $m\omega^2 x_0^2/2 = \lambda t$, and the eigenvalues $E_{\rm rel}$ of $\hat{H}_{\rm rel}$ are obtained from Eqs. (S18)-(S19) via $E_{\rm rel} = E - \lambda t$.

Since the Hamiltonian in Eq. (207) is invariant with respect to the exchange of the indices 1 and 2 (for $\epsilon = 0$), Eqs. (S18)-(S19) are invariant with respect to the simultaneous exchange of indices and inversion of the oscillator coordinate. By consequence, the pseudospinors must be either even or odd with respect to this operation, which implies $\chi_2(x) = \pm\chi_1(-x)$ for even/odd states,

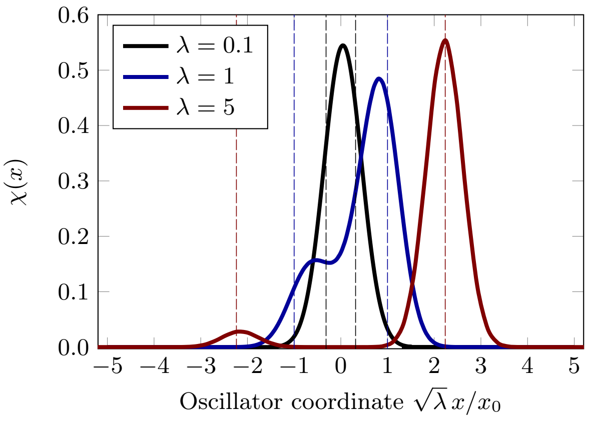


FIG. S3 Ground state solutions $\chi(x)$ of the even-parity effective Schrödinger equation for the two-site Holstein model, Eq. (S21). The curves illustrate how the wavefunction evolves upon increasing the coupling strength $\lambda$, for the adiabaticity parameter $\hbar\omega/t = 0.3$. The vertical dashed lines mark the location of the effective potential well and its mirror image.

respectively. This observation allows one to decouple Eqs. (S18)-(S19) by parity channel:

$$-\frac{\hbar^2}{2m}\frac{d^2}{dx^2}\chi + \frac{1}{2}m\omega^2(x-x_0)^2\chi \mp t\hat{P}\chi = E\chi \ , \qquad \text{(S21)}$$

where $\hat{P}\chi(x) = \chi(-x)$ is the parity operator, and the $-/+$ signs apply to the even/odd solutions, respectively. From the normalized solutions of this equation, the pseudospin components are obtained as $\chi_1(x) = \chi(x)/\sqrt{2}$ and $\chi_2(x) = \mp\chi(-x)/\sqrt{2}$, where $\mp$ is for even/odd states, respectively.

The one-dimensional Schrödinger equation (S21) contains a harmonic potential centered at $x_0$, for which one expects a Gaussian ground-state wavefunction, and a parity operator that introduces coupling with the mirror image of this function. Hence the solutions must resemble the sum of two Gaussian-like functions located near $\pm x_0$, as shown by the numerical solutions in Fig. S3.

In the strong coupling limit, the solution tends to a single displaced Gaussian, i.e., a coherent state (red curve); this scenario corresponds to the semiclassical limit. Conversely, in the weak coupling limit, the solution tends to the ground state of the oscillator centered at the origin (black curve). At intermediate coupling, the solutions consist of admixtures of Gaussian-like functions located symmetrically with respect to the origin (blue curve).

These observations suggests that a good variational ansatz for the ground state of the two-site Holstein model should include at the very least the superposition of four states:

$$|1,x_0\rangle, \quad |1,-x_0\rangle, \quad |2,x_0\rangle, \quad |2,-x_0\rangle \ , \qquad \text{(S22)}$$

where the first index denotes the electron site, and the second index denotes the ground state wavefunction of the oscillator centered at $\pm x_0$. The parity requirement reduces the possible combination of these four states to:

$$A(|1,x_0\rangle \pm |2,-x_0\rangle) + B(|2,x_0\rangle \pm |1,-x_0\rangle) \ , \qquad \text{(S23)}$$

where $\pm$ refers to even/odd states, respectively, and the coefficients $A$ and $B$ are variational parameters. This expression shows how the total wavefunction is entangled, since it cannot be written as a Born-Oppenheimer product state.

In the strong coupling limit, the contribution of $A(|1,x_0\rangle \pm |2,-x_0\rangle)$ to the wavefunction dominates over that of $B(|1,-x_0\rangle \pm |2,x_0\rangle)$, as shown by the red curve in Fig. S3. In this limit, the coherent superpositions $|1,x_0\rangle \pm |2,-x_0\rangle$ are sufficient to describe the even- and odd-parity ground states; these are precisely the states $|1\rangle \pm |2\rangle$ mentioned in Sec. XI. Using this simplified, two-state superposition, the expectation values of $\hat{H}_{\rm rel}$ for even/odd states read:

$$E^{\pm}_{\rm rel,min} = \mp t e^{-2\lambda t/\hbar\omega} + (\lambda t + \hbar\omega/2) - 2\lambda t \ , \qquad \text{(S24)}$$

where the three terms arise from the electron, phonon, and electron-phonon terms of the Hamitonian in Eq. (207), respectively. The resulting energy splitting between even and odd parity states is $\Delta E = 2te^{-2\lambda t/\hbar\omega}$.

## SUPPLEMENTAL NOTE 5: POLARONS AT FINITE TEMPERATURE

Throughout this review, we have focused on isolated polarons in their ground state at zero temperature, with the only exception being the discussion on temperature-dependent mobility of polarons in Sec. X. In the context of DFT-based calculations, the most direct way to incorporate finite temperature is through molecular dynamics simulations. Recent advances in this direction include simulations of polaron transport using molecular dynamics and machine-learned force fields (Birschitzky *et al.*, 2025) (cf. Sec. III.F), and non-adiabatic molecular dynamics simulations of polarons in transition metal oxides (Zhang *et al.*, 2021).

A many-body framework for incorporating finite-temperature effects in polaron physics is offered by Feynman's path integral formalism (cf. Sec. II.C). Building upon previous work by Ōsaka (1959) and Hellwarth and Biaggio (1999), recent efforts by Frost (2017) and Martin and Frost (2023) extended this approach to account for the presence of multiple phonon modes and to enable the calculation of temperature-dependent carrier mobilities. In these recent studies, all model parameters are determined from first-principles electronic structure calculations, thereby enhancing the predictive power of the theory.

In the context of Green's function approaches to polarons, extending the presented methods to finite temperatures involves transitioning from the real frequency

to the imaginary frequency axis using the Matsubara formalism (Fetter and Walecka, 2003). This framework naturally incorporates thermal averages via the temperature-dependent Green's function. However, a central challenge of such approaches is the necessity of performing an analytic continuation from imaginary to real frequencies in order to extract physically meaningful observables. Recent progress in this area includes the development of stochastic analytic continuation techniques (Goulko *et al.*, 2017), which have enabled the calculation of temperature-dependent mobilities within the *ab initio* diagrammatic Monte Carlo framework (cf. Sec. IV.B.2).

## SUPPLEMENTAL NOTE 6: BIPOLARONS

Bipolarons are bound states of two polarons. These composite quasiparticles can form when the lattice distortion that drives electron localization is sufficiently strong to overcome the Coulomb repulsion between the two electrons. This pairing mechanism shares some similarities with the phonon-mediated pairing of Cooper pairs in the Bardeen-Cooper-Schrieffer (BCS) theory (Alexandrov and Ranninger, 1981; Chakraverty, 1981; Lakhno, 2016). Singlet bipolarons have zero total spin, therefore they obey Bose-Einstein statistics and can undergo Bose-Einstein condensation (BEC) at sufficiently low temperatures, thus providing a possible route to superconductivity.

Historically, bipolarons attracted interest in the context of proposals for high-temperature superconductivity (Alexandrov and Ranninger, 1981), and inspired the search for oxide superconductors that eventually led to the discovery of cuprates (Bednorz and Müller, 1988).

In a two-dimensional square lattice with lattice parameter $a$ and at low bipolaron density, the critical temperature of a bipolaronic superconducting state can be estimated as $k_{\rm B}T_{\rm c} = \hbar\omega/[2(m^*/m_0)(R/a)^2]$ for $R \geq a$ and $k_{\rm B}T_{\rm c} = \hbar\omega/(2m^*/m_0)$ for $R < a$, where $\omega$, $m^*$ and $R$ are the frequency of the phonon mode coupled to this lattice, bipolaron effective mass, and bipolaron radius, respectively (Zhang *et al.*, 2023). Based on this analysis, achieving high $T_{\rm c}$ requires small and light bipolarons; these requirements are somewhat conflicting since small polarons typically carry heavy effective masses.

Calculations of bipolarons have been carried out almost exclusively for effective Hamiltonians, including the Fröhlich (Emin and Hillery, 1989) and Holstein (Chakraverty, 1981) models, and by employing variational methods (Emin and Hillery, 1989), canonical transformations (Luczak *et al.*, 1995), path integrals (Senger and Erçelebi, 2000), and quantum Monte Carlo (Hohenadler and Littlewood, 2007). A comprehensive review of bipolaron studies in continuum models is provided by Kashirina and Lakhno (2010).

Although the results often depend on the models and approximations employed, Peierls/SSH couplings have been proposed to support light small bipolarons (Zhang *et al.*, 2023), while this is not the case for Fröhlich- and Holstein-type couplings. Detailed atomistic calculations would be useful to test these promising proposals using realistic electron, phonon, and electron-phonon couplings for specific materials classes.

*Ab initio* calculations of bipolarons are scarce (Celiberti *et al.*, 2024). The main challenge here is to adequately capture the polaron-polaron interaction from first principles. The approaches reviewed in Sec. III.C address the self-interaction error of DFT, but they are not designed to handle bipolarons. Furthermore, studies on effective Hamiltonians indicate that an accurate description of electron-electron correlation is essential to allow for the formation of stable bipolarons (Kashirina and Lakhno, 2010). Therefore, developing accurate *ab initio* methods for bipolarons warrants more synergistic work at the interface between effective Hamiltonians and first-principles techniques.

## SUPPLEMENTAL NOTE 7: POLARONS OUT OF EQUILIBRIUM

Recent experiments have probed polaron formation under non-equilibrium conditions, e.g., via time-resolved X-ray diffraction of halide perovskites (Guzelturk *et al.*, 2021), ultrafast electron diffraction of two-dimensional materials (Britt *et al.*, 2024; de Cotret *et al.*, 2022), and transient absorption spectroscopy in halide perovskites (Wright *et al.*, 2021) and transition-metal oxides (Johnston *et al.*, 2025; Tian *et al.*, 2025). These studies provide a strong motivation for developing theoretical frameworks that capture the time evolution of polaron localization and dynamics.

At the formal level, work in this direction was undertaken by Stefanucci *et al.* (2023), who formulated an *ab initio* nonequilibrium electron-phonon theory starting from the Kadanoff-Baym equations. This framework recovers the Hedin-Baym theory (Giustino, 2017) in the equilibrium limit, and includes a term that is similar to the polaron self-energy identified in Sec. V of this review. The main difference between the approach of Stefanucci *et al.* (2023) and the techniques reviewed in this article is that, in their formulation, the electron-phonon matrix element that drives the formation of polarons is not screened. Further work will be needed to better understand the origin and implications of this difference.

Direct *ab initio* calculations of polaron dynamics include those based on time-dependent DFT (TDDFT) (Marques and Gross, 2006) in supercells, such as for example the study of polaron-assisted hole transfer mechanism of photoinduced water dissociation on $TiO_2$ (You *et al.*, 2024), or the study of exciton-polaron dynamics and recombination in $Fe_2O_3$ (Rassouli *et al.*, 2024).

TDDFT-based supercell approaches have also been used to investigate light-driven polaron dynamics from first principles; for example, Wang *et al.* (2023) showed that driving phonons that participate in the polaronic distortion can modulate hopping barriers, thereby controlling transport properties. Beyond supercell calculations, polaron formation and charge-transfer dynamics have also been studied within a two-site Holstein model (Panhans *et al.*, 2023) relevant to transport in organic crystals (Hutsch *et al.*, 2022), and a time-dependent version of the *ab initio* polaron equations of Sec. VI.C has recently been proposed (Garcia-Herrero *et al.*, 2025). Given the growing number of experiments probing real-time dynamics of polarons, we can anticipate more theoretical and computational work in this area going forward.

## REFERENCES


Abramovitch, D. J., J. Coulter, S. Beck, and A. Millis (2025), "Electron-phonon coupling in correlated metals: A dynamical mean-field theory study," Phys. Rev. B **112**, 075113.

Adelstein, N., J. B. Neaton, M. Asta, and L. C. De Jonghe (2014), "Density functional theory based calculation of small-polaron mobility in hematite," Phys. Rev. B **89**, 245115.

Alexandrov, A., and J. Ranninger (1981), "Theory of bipolarons and bipolaronic bands," Phys. Rev. B **23**, 1796.

Bednorz, J. G., and K. A. Müller (1988), "Perovskite-type oxides—the new approach to high-$T_c$ superconductivity," Rev. Mod. Phys. **60**, 585.

Birschitzky, V. C., L. Leoni, M. Reticcioli, and C. Franchini (2025), "Machine learning small polaron dynamics," Phys. Rev. Lett. **134**, 216301.

Britt, T. L., F. Caruso, and B. J. Siwick (2024), "A momentum-resolved view of polaron formation in materials," npj Comput. Mater. **10**, 178.

Carey, J. J., J. A. Quirk, and K. P. McKenna (2021), "Hole polaron migration in bulk phases of $TiO_2$ using hybrid density functional theory," J. Phys. Chem. C **125**, 12441.

Celiberti, L., D. Fiore Mosca, G. Allodi, L. V. Pourovskii, A. Tassetti, P. C. Forino, R. Cong, E. Garcia, P. M. Tran, R. De Renzi, *et al.* (2024), "Spin-orbital Jahn-Teller bipolarons," Nat. Commun. **15**, 2429.

Chakraverty, B. (1981), "Bipolarons and superconductivity," J. Phys. France **42**, 1351.

de Cotret, L. P. R., M. R. Otto, J.-H. Pöhls, Z. Luo, M. G. Kanatzidis, and B. J. Siwick (2022), "Direct visualization of polaron formation in the thermoelectric SnSe," Proc. Natl. Acad. Sci. U.S.A. **119**, e2113967119.

Dai, Z., and F. Giustino (2024), "Identification of large polarons and exciton polarons in rutile and anatase polymorphs of titanium dioxide," Proc. Natl. Acad. Sci. U.S.A. **121**, e2414203121.

Deskins, N. A., and M. Dupuis (2007), "Electron transport via polaron hopping in bulk $TiO_2$: A density functional theory characterization," Phys. Rev. B **75**, 195212.

Emin, D., and M. Hillery (1989), "Formation of a large singlet bipolaron: application to high-temperature bipolaronic superconductivity," Phys. Rev. B **39**, 6575.

Eyring, H. (1935), "The activated complex in chemical reactions," J. Chem. Phys. **3**, 107.

Falletta, S., and A. Pasquarello (2023), "Polaron hopping through piecewise-linear functionals," Phys. Rev. B **107**, 205125.

Fetter, A., and J. Walecka (2003), *Quantum theory of many-particle systems* (Dover, New York).

Frost, J. M. (2017), "Calculating polaron mobility in halide perovskites," Phys. Rev. B **96**, 195202.

Garcia-Herrero, V., C. Emeis, J. Lafuente-Bartolome, F. Giustino, and F. Caruso (2025), "Watching polarons form in real time," Unpublished.

Giustino, F. (2017), "Electron-phonon interactions from first principles," Rev. Mod. Phys. **89**, 015003.

Goldey, M. B., N. P. Brawand, M. Voros, and G. Galli (2017), "Charge transport in nanostructured materials: implementation and verification of constrained density functional theory," J. Chem. Theory Comput. **13**, 2581.

Goulko, O., A. S. Mishchenko, L. Pollet, N. Prokof'ev, and B. Svistunov (2017), "Numerical analytic continuation: Answers to well-posed questions," Phys. Rev. B **95**, 014102.

Guzelturk, B., T. Winkler, T. W. J. Van de Goor, M. D. Smith, S. A. Bourelle, S. Feldmann, M. Trigo, S. W. Teitelbaum, H.-G. Steinrück, G. A. de la Pena, R. Alonso-Mori, D. Zhu, T. Sato, H. I. Karunadasa, M. F. Toney, F. Deschler, and A. M. Lindenberg (2021), "Visualization of dynamic polaronic strain fields in hybrid lead halide perovskites," Nat. Mater. **20**, 618.

Hellwarth, R. W., and I. Biaggio (1999), "Mobility of an electron in a multimode polar lattice," Phys. Rev. B **60**, 299.

Hohenadler, M., and P. B. Littlewood (2007), "Quantum Monte Carlo results for bipolaron stability in quantum dots," Phys. Rev. B **76**, 155122.

Hutsch, S., M. Panhans, and F. Ortmann (2022), "Charge carrier mobilities of organic semiconductors: ab initio simulations with mode-specific treatment of molecular vibrations," npj Computational Materials **8**, 228.

Imada, M., A. Fujimori, and Y. Tokura (1998), "Metal-insulator transitions," Rev. Mod. Phys. **70**, 1039.

Johnston, C. R., R. Speelman, A. Arcidiacono, C. M. Bridgewater, L. Rassouli, X. Ma, I. Vargas-Hurlston, J. Kupferberg, L. E. Martin, A. B. F. Martinson, M. Dupuis, F. M. Geiger, and S. B. King (2025), "Watching polarons dance: Coherent carrier-phonon coupling in hematite revealed by transient absorption spectroscopy," ChemRxiv doi:10.26434/chemrxiv-2025-lgzgr.

Kashirina, N. I., and V. D. Lakhno (2010), "Large-radius bipolaron and the polaron-polaron interaction," Phys. Usp. **53**, 431.

Lafuente-Bartolome, J., C. Lian, and F. Giustino (2024), "Topological polarons in halide perovskites," Proc. Natl. Acad. Sci. U.S.A. **121**, e2318151121.

Lakhno, V. (2016), "Cooper pairs and bipolarons," Mod. Phys. Lett. B **30**, 1650365.

Landau, L. D. (1932a), "A theory of energy transfer. II," Phys. Z. Sowjetunion **2**, 46.

Landau, L. D. (1932b), "A theory of energy transfer on collisions," Phys. Z. Sowjetunion **1**, 88.

Luczak, F., F. Brosens, and J. Devreese (1995), "Formation of large bipolarons," Phys. Rev. B **52**, 12743.

Marques, M. A., and E. K. Gross (2006), *Time-dependent density functional theory* (Springer Berlin, Heidelberg).

Martin, B. A. A., and J. M. Frost (2023), "Multiple phonon modes in Feynman path-integral variational polaron mobil-

ity," Phys. Rev. B **107**, 115203.

Mott, N. F. (1968), "Metal-insulator transition," Rev. Mod. Phys. **40**, 677.

Newton, M. D. (1991), "Quantum chemical probes of electron-transfer kinetics: the nature of donor-acceptor interactions," Chem. Rev. **91**, 767.

Ōsaka, Y. (1959), "Polaron state at a finite temperature," Prog. Theor. Phys. **22**, 437.

Palermo, G., S. Falletta, and A. Pasquarello (2024), "Migration of hole polarons in anatase and rutile $TiO_2$ through piecewise-linear functionals," Phys. Rev. B **110**, 235205.

Panhans, M., S. Hutsch, and F. Ortmann (2023), "Insight on charge-transfer regimes in electron-phonon coupled molecular systems via numerically exact simulations," Communications Physics **6**, 125.

Park, H., N. Kumar, M. Melander, T. Vegge, J. M. Garcia Lastra, and D. J. Siegel (2018), "Adiabatic and nonadiabatic charge transport in Li–S batteries," Chem. Mater. **30**, 915.

Rassouli, L., M. Shakiba, A. V. Akimov, X. Ma, and M. Dupuis (2024), "Excitons in hematite fe2o3: Short-time dynamics from td-dft and non-adiabatic dynamics theories," J. Phys. Chem. C **128**, 13681.

Senger, R. T., and A. Erçelebi (2000), "Path-integral approximation on the stability of large bipolarons in quasi-one-dimensional confinement," Phys. Rev. B **61**, 6063.

Sio, W. H., C. Verdi, S. Poncé, and F. Giustino (2019a), "Ab initio theory of polarons: Formalism and applications," Phys. Rev. B **99**, 235139.

Sio, W. H., C. Verdi, S. Poncé, and F. Giustino (2019b), "Polarons from first principles, without supercells," Phys. Rev. Lett. **122**, 246403.

Stefanucci, G., R. van Leeuwen, and E. Perfetto (2023), "In and out-of-equilibrium ab initio theory of electrons and phonons," Phys. Rev. X **13**, 031026.

Tian, L., M. Sachs, L. Verga, V. Kunzelmann, A. Kafizas, I. Sharp, S. Cushing, A. Walsh, and J. Durrant (2025), "Optical spectroscopic determination of photoexcited small-polaron hopping in transition metal oxide photocatalysts," ChemRxiv doi:10.26434/chemrxiv-2025-bhf0z.

Wang, H.-M., X.-B. Liu, S.-Q. Hu, D.-Q. Chen, Q. Chen, C. Zhang, M.-X. Guan, and S. Meng (2023), "Giant acceleration of polaron transport by ultrafast laser-induced coherent phonons," Sci. Adv. **9**, eadg3833.

Wimmer, E., W. Wolf, J. Sticht, P. Saxe, C. B. Geller, R. Najafabadi, and G. A. Young (2008), "Temperature-dependent diffusion coefficients from ab initio computations: Hydrogen, deuterium, and tritium in nickel," Phys. Rev. B **77**, 134305.

Wright, A. D., L. R. V. Buizza, K. J. Savill, G. Longo, H. J. Snaith, M. B. Johnston, and L. M. Herz (2021), "Ultrafast excited-state localization in $Cs_2AgBiBr_6$ double perovskite," J. Phys. Chem. Lett. **12**, 3352.

Wu, F., and Y. Ping (2018), "Combining Landau–Zener theory and kinetic Monte Carlo sampling for small polaron mobility of doped $BiVO_4$ from first-principles," J. Mater. Chem. A **6**, 20025.

You, P., D. Chen, X. Liu, C. Zhang, A. Selloni, and S. Meng (2024), "Correlated electron–nuclear dynamics of photoinduced water dissociation on rutile tio2," Nat. Mater. **23**, 1100.

Zener, C. (1932), "Non-adiabatic crossing of energy levels," Proc. R. Soc. London, Ser. A **137**, 696.

Zhang, C., J. Sous, D. R. Reichman, M. Berciu, A. J. Millis, N. V. Prokof'ev, and B. V. Svistunov (2023), "Bipolaronic high-temperature superconductivity," Phys. Rev. X **13**, 011010.

Zhang, L., W. Chu, C. Zhao, Q. Zheng, O. V. Prezhdo, and J. Zhao (2021), "Dynamics of photoexcited small polarons in transition-metal oxides," J. Phys. Chem. Lett. **12**, 2191.
